# Supplementary material for: Model Comparison for Fast Domain Adaptation in Table Service Scenario
Source: arXiv:2403.05092 source file (2024-03-08)
Supplement: Supplementary file 1 [file root_supp.tex]

% \subsubsection{classification to detection}
% 먼저 문제를 classification 방식으로 푸는 방법과 detection 방법으로 푸는 방법을 비교해보았다. 각 추천 서비스는 해당 서비스의 원인이 되는 영역이 있기에 이를 바탕으로 detection방법을 학습해보았고, 영역정보를 무시하고 classification방법을 학습했다.

% \begin{table}[tb]
% \caption{4종의 학습과 테스트에 사용된 이미지의 수와 정답의 빈도 }
% \label{tab:a}
% \begin{center}
% \begin{tabular}{|c||c|c|c|c|}
% \hline
% approach   & num of params   & accuracy      & f1        & roc    \\
% \hline
% image      & 100             & 2440          & 2301      & 627              \\
% % \hline
% test       & 100             & 9848          & 6622      & 3613             \\
% \hline
% \end{tabular}
% \end{center}
% \end{table}

% 결과를 보면 cls의 결과가 det보다 좋았다.
